# Supplementary material for: Guided Depth Super-Resolution by Deep Anisotropic Diffusion
Source: arXiv:2211.11592 source file (2023-03-28)
Supplement: Supplementary file 1 [file additional_metrics.tex]

\begin{table}[h]
\centering
\footnotesize
 % \resizebox{0.475\textwidth}{!}{%
\begin{tabularx}{0.40\textwidth}{l| YYY}
 & \multicolumn{3}{c}{Middlebury} & \multicolumn{3}{c}{NYUv2} \midrule \\
 [\%] & V-err & E-err & MAPE \\ \midrule 
 MSG          & ? & ? & ?  \\
 DKN          & ? & ? & ?  \\
 FDKN         & ? & ? & ?  \\
 PMBA         & ? & ? & ?  \\
 FDSR         & ? & ? & ?  \\
 LGR          & ? & ? & ?  \\
 DADA         & ? & ? & ?
\end{tabularx}%
 % }%\usepackage{adjustbox}
\caption{}
\label{tab:encoders}
\end{table}
