# Supplementary material for: Guided Depth Super-Resolution by Deep Anisotropic Diffusion
Source: arXiv:2211.11592 source file (2023-03-28)
Supplement: Supplementary file 2 [file additional_metrics_v2.tex]

\begin{table}[h]
\centering
\footnotesize
\vspace{-0.075cm}
 \resizebox{0.45\textwidth}{!}{%
\begin{tabular}{l| ccc}
 \multicolumn{1}{c}{} & \textbf{Middlebury} & \textbf{NYUv2} & \textbf{DIML}  \\ 
 \multicolumn{1}{c}{in $[\%]$} &       MAPE/VE/EE & MAPE/VE/EE & MAPE/VE/EE  \\ \midrule  
 MSG          &  0.8 / 1.7 / 14.7 &  1.9 / 3.0 / 49.8 &  0.9 / 1.2 / 24.8 \\
 DKN          &  1.2 / 2.7 / 21.9 &  2.4 / 4.4 / 55.8 &  1.4 / 2.2 / 32.3 \\
 FDKN         &  1.2 / 2.6 / 21.7 &  2.4 / 4.5 / 55.7 &  1.4 / 2.2 / 34.3 \\
 PMBA         &  1.9 / 4.1 / 35.7 &  2.7 / 5.2 / 57.4 &  0.8 / 1.2 / 25.0 \\
 FDSR         &  1.6 / 3.7 / 21.6 &  3.4 / 7.2 / 63.4 &  1.6 / 2.5 / 36.3 \\
 LGR          &  0.6 / 1.2 / 12.8 &  1.8 / 2.7 / 49.0 &  0.9 / 1.3 / 26.7 \\
 DADA         &  \textbf{0.5} / \textbf{0.9} / \textbf{8.1} &  \textbf{1.6} / \textbf{2.4} / \textbf{44.3} &  \textbf{0.7} / \textbf{0.9} / \textbf{19.7}
\end{tabular}%
 }%\usepackage{adjustbox}
 \vspace{-0.1cm}
\caption{Middlebury, scale x32, all numbers are in [\%].}
\vspace{-0.2cm}
\label{tab:new_metrics}
\end{table}
